# Supplementary material for: Aligning Robot Navigation Behaviors with Human Intentions and Preferences
Source: arXiv:2409.18982 source file (2024-09-16)
Supplement: Supplementary file 1 [file appendix.tex]

% Be sure to set \appendix or \appendices in structural/body.tex
\chapter{Appendix Name}
Text here.
\section{Appendix section}
Text here.
\subsection{Appendix section}
Text here.
\subsubsection{Appendix section}
Text here.
\chapter{Another Appendix}
